# Supplementary material for: Reactive Optimizers
Source: arXiv:2610.33826 source file (2026-11-04)
Supplement: Supplementary file 1 [file appendix.tex]

% generated by scripts/blog_to_tex.py from the blog's share/reactive-optimizers.html; edit the generator
